# Supplementary material for: InterLUDE: Interactions between Labeled and Unlabeled Data to Enhance Semi-Supervised Learning
Source: arXiv:2403.10658 source file (2024-03-15)
Supplement: Supplementary file 1 [file supplement.tex]

\section{Discussion Embedding Fusion}
This section provides the perspective from task complexity to explain the embedding fusion works in SSL settings. 
In general, the definition of information entropy of a specific task can be formulated as \cite{Li2022PN}:
\begin{equation}
\label{LiTaskEntropy}
H(\mathcal{T};\boldsymbol{X})=-\sum_{\boldsymbol{Y} \in \mathcal{Y}}p(\boldsymbol{Y}|\boldsymbol{X})\log{p(\boldsymbol{Y}|\boldsymbol{X})}  
\end{equation}
The images $\boldsymbol{X}$ within the dataset are expected to be mutually independent, as well as the labels $\boldsymbol{Y}$. Nevertheless, the independence between $\boldsymbol{X}$ and $\boldsymbol{Y}$ is compromised due to the association between a data sample $x$ and its corresponding label $y$. This correlation results in the conditional distribution of $\boldsymbol{Y}$ given $\boldsymbol{X}$ being reliant on the joint distribution of $\boldsymbol{X}$ and $\boldsymbol{Y}$. In the absence of knowledge regarding the joint distribution of $\boldsymbol{X}$ and $\boldsymbol{Y}$, determining the conditional distribution of $\boldsymbol{Y}$ and $\boldsymbol{X}$ becomes impossible. To mitigate this issue, we introduce some allowances for the distribution of $\boldsymbol{X}$ and $\boldsymbol{Y}$. Employing various techniques like Box-Cox transformation, log transformation, etc., \cite{Box64, Feng2014}, enables us to transform the unknown distributions of $\boldsymbol{X}$ and $\boldsymbol{Y}$ to approximate normality. Following this approximate transformation, the distributions of $\boldsymbol{X}$ and $\boldsymbol{Y}$ can be represented as:
\begin{equation}\label{SlackXY}
 %\boldsymbol{X}\sim \mathcal{N}(\mu_{X}, \sigma^{2}_{X}  ), %\boldsymbol{Y}\sim \mathcal{N}(\mu_{Y}, \sigma^{2}_{Y}  )
  \boldsymbol{X}\sim \mathcal{N}( \boldsymbol{\mu_{X}}, \boldsymbol{\Sigma_{X}}  ), \boldsymbol{Y}\sim \mathcal{N}(\boldsymbol{\mu_{Y}}, \boldsymbol{\Sigma_{Y}}  )
\end{equation}
where $\boldsymbol{\mu_{X}}$ and $\boldsymbol{\Sigma_{X}}$ represent the mean of the dataset and the corresponding labels, respectively, while the $\boldsymbol{\Sigma_{X}} $ and $\boldsymbol{\Sigma_{Y}} $ mean the covariance matrix of the dataset and label, respectively.
\iffalse
\begin{equation}
\begin{split}
  &\boldsymbol{{\mu}_{X} }=\mathbb{E}[\boldsymbol{X}]=(\mathbb{E}[x_{1}], \mathbb{E}[x_{2}],...,\mathbb{E}[x_{k}]])^{T} \\
  &\boldsymbol{{\mu}_{Y} }=\mathbb{E}[\boldsymbol{Y}]=(\mathbb{E}[y_{1}], \mathbb{E}[y_{2}],...,\mathbb{E}[y_{k}]])^{T} \\
  &\boldsymbol{\Sigma_{X}}=\mathbb{E}[(\boldsymbol{X}-\boldsymbol{{\mu}_{X}})(\boldsymbol{X}-\boldsymbol{{\mu}_{X}})^{T}] \\
 & \boldsymbol{\Sigma_{Y}}=\mathbb{E}[(\boldsymbol{Y}-\boldsymbol{{\mu}_{Y}})(\boldsymbol{Y}-\boldsymbol{{\mu}_{Y}})^{T}]
\end{split}
\end{equation}
$k$ is the number of samples in the dataset, and $T$ represents the transpose of the matrix.
\fi
With appropriate transformation, the $\boldsymbol{X}$ and $\boldsymbol{Y}$ follow a multivariate normal distribution. Consequently, the conditional distribution of $\boldsymbol{Y}$ given $\boldsymbol{X}$ adheres to a normal distribution \cite{Mood1950, Johnson1995}, which can be formulated as:
\begin{equation}
\boldsymbol{Y}|\boldsymbol{X}\sim \mathcal{N}(\mathbb{E}({\boldsymbol{Y}|\boldsymbol{X}=\boldsymbol{x}}), var(\boldsymbol{Y}|\boldsymbol{X}=\boldsymbol{x}))
\end{equation}
where $\mathbb{E}({\boldsymbol{Y}|\boldsymbol{X}=\boldsymbol{x}})$ is the mean of the label set $\boldsymbol{Y}$ given a sample $\boldsymbol{X}=\boldsymbol{x}$ from the feasible space, and $var(\boldsymbol{Y}|\boldsymbol{X}=\boldsymbol{x})$ is the variance. The conditional mean $\mathbb{E} (\boldsymbol{Y}|\boldsymbol{X}=\boldsymbol{x}) ] $ and conditional variance $var(\boldsymbol{Y}|\boldsymbol{X}=X)$ can be quantified as: 
\begin{equation}
\boldsymbol{\mu}_{\boldsymbol{Y}|\boldsymbol{X}=\boldsymbol{x}}=\mathbb{E}[(\boldsymbol{Y}|\boldsymbol{X}=\boldsymbol{x}) ] =\boldsymbol{{\mu}_{Y}}+\boldsymbol{\Sigma_{YX}}\boldsymbol{{\Sigma}^{-1}_{X}}(\boldsymbol{x}-\boldsymbol{\mu_{X}})
\end{equation}
\begin{equation}
\boldsymbol{\Sigma}_{{\boldsymbol{Y|X}}=\boldsymbol{x}}=var(\boldsymbol{Y}|\boldsymbol{X}=\boldsymbol{x})=\boldsymbol{\Sigma_{Y}-\Sigma_{YX}{\Sigma}^{-1}_{X}\Sigma_{XY}}
\end{equation}
where $\boldsymbol{\Sigma_{YX}}$ and $\boldsymbol{\Sigma_{XY}}$ are the cross-covariance matrices between $\boldsymbol{Y}$ and $\boldsymbol{X}$, and between $\boldsymbol{X}$ and $\boldsymbol{Y}$, respectively, and $\boldsymbol{\Sigma^{-1}_{X}}$ denotes the inverse of the covariance matrix of $\boldsymbol{X}$.

\noindent As we have the distribution of $\boldsymbol{Y|X}$, we shall obtain the task entropy:
\begin{equation}
\label{LITaskEntropyQuantitive}
\resizebox{0.48\textwidth}{!}{$ \begin{split}
H(\mathcal{T};\boldsymbol{X})=&-\sum_{\boldsymbol{Y} \in \mathcal{Y}}p(\boldsymbol{Y}|\boldsymbol{X})\log{p(\boldsymbol{Y}|\boldsymbol{X})}  \\
=&-\mathbb{E}[\log p(\boldsymbol{Y}|\boldsymbol{X})] \\
=& -\mathbb{E}[\log [(2\pi)^{-K/2}|\boldsymbol{\Sigma_{Z}}|^{-1/2}\exp(-\frac{1}{2} \boldsymbol{(Z - \mu_{Z})}^{T} \boldsymbol{\Sigma}^{-1}_{\boldsymbol{Z}}(\boldsymbol{Z} - \boldsymbol{\mu_{Z}}))]] \\
=&\frac{K}{2} \log (2\pi) + \frac{1}{2} \log|\boldsymbol{\Sigma_{Z}}|+\frac{1}{2} \mathbb{E}[{(\boldsymbol{Z} - \boldsymbol{\mu}_{\boldsymbol{Z}})}^{T} \Sigma^{-1}_{\boldsymbol{\boldsymbol{Z}}}(\boldsymbol{Z} - \boldsymbol{\mu}_{\boldsymbol{Z}})] \\
=&\frac{K}{2} (1+ \log (2\pi)) + \frac{1}{2} \log |\boldsymbol{\Sigma_{Z}}|
\end{split} $}
\end{equation}
where we use ${\boldsymbol{Z}}$ to represent $\boldsymbol{Y|X}$, and 
\begin{equation}
\resizebox{0.45\textwidth}{!}{$ \begin{split}
 \mathbb{E}[{(\boldsymbol{Z} - \boldsymbol{\mu}_{\boldsymbol{Z}})}^{T} \Sigma^{-1}_{\boldsymbol{\boldsymbol{Z}}}(\boldsymbol{Z} - \boldsymbol{\mu}_{\boldsymbol{Z}})]
=& \mathbb{E}[tr((\boldsymbol{Z} - \boldsymbol{\mu}_{\boldsymbol{Z}})^{T} \Sigma^{-1}_{\boldsymbol{\boldsymbol{Z}}}(\boldsymbol{Z} - \boldsymbol{\mu}_{\boldsymbol{Z}}))] \\
=& K
\end{split} $}
\end{equation} where $K$ is the number of data samples in the dataset. Therefore, for a specific dataset, we can find that the task entropy is only related to the variance of the $\boldsymbol{Y|X}$. However, when operations are applied to the embeddings within the latent space, the task entropy is defined as \cite{Yu2023PN}:
\begin{equation}
\label{latentEntropyChange}
H(\mathcal{T};\boldsymbol{X}+\boldsymbol{\epsilon}) = H(\boldsymbol{Y};\boldsymbol{X}+\boldsymbol{\epsilon}) - H(\boldsymbol{X}) 
\end{equation}
where $\boldsymbol{\epsilon}$ is the additive operation applied to the embeddings. $H(\mathcal{T};\boldsymbol{X}+\boldsymbol{\epsilon}) $ elaborates on the entropy of a learning system in the context of additive operations applied to embeddings, exemplified by the embedding fusion for SSL introduced in the following section. Because the operations are conducted on the embeddings within the latent space rather than on the raw images, EQ. \ref{latentEntropyChange} differs from EQ. \ref{LiTaskEntropy}. Here, $H(\boldsymbol{X})$ represents the dataset's entropy, while $H(\boldsymbol{Y};\boldsymbol{X}+\boldsymbol{\epsilon})$ denotes the joint entropy of the label and dataset with an additive term $\boldsymbol{\epsilon}$.

Therefore, there are two approaches to achieving entropy reduction: the first involves operating on the image level, utilizing the definition provided in \ref{LiTaskEntropy}, while the other involves operating on the embedding level, employing the definition from \ref{latentEntropyChange}. After comparing the conclusions in the works \cite{Li2022PN, Yu2023PN}, we propose embedding fusion that operates in the latent space, as this embedding-level operation could be a more effective approach.

\section{Embedding Fusion in SSL}

Building upon the concepts outlined in the previous section, we explore the entropy reduction for SSL tasks. The primary challenge lies in the presence of a substantial amount of unlabeled data samples and a severely limited number of labeled data samples in SSL tasks. This scenario markedly differs from previous studies where each data sample had a true label \cite{Li2022PN, Yu2023PN}. In this work, we utilize pseudo labels as the substitutes for true labels of the unlabeled data samples. For SSL tasks, the available dataset includes a limited number of labeled samples and a large number of unlabeled samples, represented as $\boldsymbol{X}=\left \{ \mathcal{L} \cup  \mathcal{U}\right \}$, and the labels includes the true labels of the labeled data and pseudo labels of the unlabeled data, represented as $ \hat{\boldsymbol{Y} }=\left \{ Y_{\mathcal{L}} \cup \hat{Y}_{\mathcal{U}} \right \} $, where $Y_{\mathcal{L}} $ is the true label, and $\hat{Y}_{\mathcal{U}}$ is the pseudo label predicted by the trained model. It is important to note that the quality of the pseudo label relies on the predictive capability of the trained model.

Since we adopt only linear operations on the embeddings, we can employ a linear transformation matrix, denoted as $A$, to design the embedding fusion strategy. The formulation of the entropy change resulting from operating the embedding fusion can be expressed as: 
\begin{equation} \label{LinearNosieFormulaAppendix}
\resizebox{0.47\textwidth}{!}{$ \begin{split}
 \bigtriangleup S(\mathcal{T},A\boldsymbol{X } )
= & [H(\hat{\boldsymbol{Y}};\boldsymbol{X}) - H(\boldsymbol{X})] -[ H(\hat{\boldsymbol{Y_{e}}};\boldsymbol{X}+A\boldsymbol{X})- H(\boldsymbol{X} )]\\
=&H(\hat{\boldsymbol{Y}};\boldsymbol{X}) - H(\hat{\boldsymbol{Y_{e}}};\boldsymbol{X}+A\boldsymbol{X}) \\
=&H(\hat{\boldsymbol{Y}}|\boldsymbol{X})+H(\boldsymbol{X}) - [H(\hat{\boldsymbol{Y_{e}}}|(I+A)\boldsymbol{X})+H((I+A)\boldsymbol{X}) ]
\end{split}  $}
\end{equation}
where the first term within $[\cdot]$ represents the entropy of the learning system in the SSL learning task, while the second term within $[\cdot]$ denotes the entropy of the learning system when employing embedding fusion in the SSL learning task. $\hat{\boldsymbol{Y}}$ comprises the pseudo labels predicted by the trained model, while $\hat{\boldsymbol{Y_{e}}}$ comprises the pseudo labels predicted by the trained model equipped with embedding fusion. $\hat{\boldsymbol{Y}}$ is different from $\hat{\boldsymbol{Y_{e}}}$.
As long as the entropy change $\bigtriangleup S(\mathcal{T}, A\boldsymbol{X } )$ is greater than 0, we can realize entropy reduction. Borrow the conclusion in EQ. \ref{LITaskEntropyQuantitive} and knowledge of conditional entropy \cite{MacKay2003Information}, we can obtain:
\begin{equation} 
\label{entropychange}
\resizebox{0.47\textwidth}{!}{$ \begin{split}
 \bigtriangleup S(\mathcal{T},A\boldsymbol{X } )
=&\frac{1}{2} \log|\boldsymbol{\Sigma_{\hat{Y}|X}}| + \frac{1}{2} \log|\boldsymbol{\Sigma_{X}}| - \frac{1}{2} \log|\boldsymbol{\Sigma}_{\boldsymbol{\hat{Y}_e}|(I+A)\boldsymbol{X}}| - \frac{1}{2} \log|\boldsymbol{\Sigma}_{(I+A)\boldsymbol{X}}| \\
=&\frac{1}{2} \log \frac{|\boldsymbol{\Sigma_{X}}||\boldsymbol{\Sigma_{\hat{Y}|X}}|}{|\boldsymbol{\Sigma}_{(I+A)\boldsymbol{X}}||\boldsymbol{\Sigma}_{\boldsymbol{\hat{Y}_e}|(I+A)\boldsymbol{X}}|} \\
=&\frac{1}{2} \log \frac{ 1 }{|I+A|^{2}} + \frac{1}{2} \log \frac{|\boldsymbol{\Sigma_{\hat{Y}}}-\boldsymbol{\Sigma_{\hat{Y}X}}{\boldsymbol{\Sigma_{X}^{-1}}}\boldsymbol{\Sigma_{X\hat{Y}}}|}{|\boldsymbol{\Sigma_{\hat{Y}_e}-\Sigma_{ {\hat{Y}}_e X}}\boldsymbol{\Sigma^{-1}_{X}}\boldsymbol{\Sigma_{X\hat{Y}_e}}|}\\
=&\frac{1}{2} \log \frac{ 1 }{|I+A|^{2}} + \mathcal{M}( \hat{\theta}, \hat{\theta}_e(A) )\\
=&-\log|I+A| + \mathcal{M}( \hat{\theta}, \hat{\theta}_e(A) )
\end{split}  $}
\end{equation}
where $\hat{\theta}$ and $\hat{\theta}_{e}$ are the model parameters with and without embedding fusion, and the conditional variance matrix of $\boldsymbol{\Sigma}_{\boldsymbol{\hat{Y}_{e}}|(I+A)\boldsymbol{X}}$ is quantified as
$\boldsymbol{\Sigma_{\hat{Y}_{e}}}-\boldsymbol{\Sigma}_{\boldsymbol{\hat{Y}_{e}}((I+A)\boldsymbol{X} )}\boldsymbol{\Sigma}^{-1}_{(I+A)\boldsymbol{X} }\boldsymbol{\Sigma}_{((I+A)\boldsymbol{X})\boldsymbol{Y}_{e}}$. $\boldsymbol{\Sigma}_{\boldsymbol{\hat{Y}_{e}}((I+A)\boldsymbol{X} )}\boldsymbol{\Sigma}^{-1}_{(I+A)\boldsymbol{X} }\boldsymbol{\Sigma}_{((I+A)\boldsymbol{X})\boldsymbol{Y}_{e}}$ is simplified with covariance matrix property to $\boldsymbol{\Sigma_{\hat{Y}_e}-\Sigma_{ {\hat{Y}}_e X}}\boldsymbol{\Sigma^{-1}_{X}}\boldsymbol{\Sigma_{X\hat{Y}_e}}$. We use $\mathcal{M}( \hat{\theta}, \hat{\theta}_e(A) )$ to represent the second term, i.e., $\frac{1}{2} \log \frac{|\boldsymbol{\Sigma_{\hat{Y}}}-\boldsymbol{\Sigma_{\hat{Y}X}}{\boldsymbol{\Sigma_{X}^{-1}}}\boldsymbol{\Sigma_{X\hat{Y}}}|}{|\boldsymbol{\Sigma_{\hat{Y}_e}-\Sigma_{ {\hat{Y}}_e X}}\boldsymbol{\Sigma^{-1}_{X}}\boldsymbol{\Sigma_{X\hat{Y}_e}}|}$ in entropy change. The first term shows the influence of data on entropy change. The second term signifies that the entropy change is influenced by the disparity between pseudo-labels and true labels for the unlabeled data. Note if the trained model has ideal prediction ability, then the predicted labels $\boldsymbol{\hat{Y}_{e}}$ equals $\boldsymbol{\hat{Y}}$.

As stated in the paper, we also need to consider the constraints, we can formulate entropy change as an optimization problem:
\begin{equation} \label{LinearNosieOptimizationAppendix}
\begin{split}
&   \max_{A}  \bigtriangleup S(\mathcal{T},A\boldsymbol{X } ) \\
&s.t. \ rank(I+A)=k \\
&\ \quad  \left [ I+A \right ]_{ii} > \left [ I+A \right ]_{ij}, i \ne j \\
& \ \quad  \left \| \left [ I+A \right ]_{i}   \right \|_{1} = 1 
\end{split}
\end{equation}
The key to determining whether the embedding fusion is beneficial or not lies in the matrix of $A$. The most crucial step is to ensure that $I+A$ is of full rank. This ensures that no information from the images will be eliminated after embedding fusion.

In fact, a design space exists for embedding fusion within the variable $A$. However, it's important to emphasize that, as the entropy change is determined by two terms, as stated in EQ. \ref{entropychange}, we can directly control the first term using matrix theory, but controlling the complex second term directly is not feasible. Furthermore, the viable design space for the first term of $A$ is constrained by the presence of the second term. In this work, we employ the circular shift \cite{zhang2020CS} as our chosen embedding fusion strategy. The circular shift adapted in our work can be formulated as:
\begin{equation}
\begin{split}
 I+A =& \begin{bmatrix}
 1 &  &  &  &\\
  & 1 &  & &\\
  &  & . & &\\
  &  &  & 1& \\
  &  &  & &1
\end{bmatrix} + \begin{bmatrix}
 -\alpha & \alpha  &  &  &\\
  & . & .&  &\\
  &  & . &. &\\
  &  &  & . & \alpha\\
\alpha  &  &  & &-\alpha
\end{bmatrix}  \\
 =&
\begin{bmatrix} 
1-\alpha &\alpha  &  &  &\\
  & . & . & &\\
  &  & . &. &\\
  &  &  & .& \alpha \\
\alpha  &  &  & &1-\alpha
\end{bmatrix}
\end{split}
\end{equation}
where $\alpha$ is the embedding fusion strength. We can adjust the embedding fusion strength to make the $ \bigtriangleup S(\mathcal{T}, A\boldsymbol{X } ) > 0$, therefore realizing entropy reduction.


\section{Additional Experiments}
\label{Additional Experiments}
\begin{figure}[htb]
  \centering
 \includegraphics[width= 8.5cm]{figs/Ablation_FusionStrategy_CNN_CIFA10.pdf}
%  \vspace{2.0cm}
  \label{FusionStrategy}
  \caption{Abalation on Embedding Fusion Strategy}
\end{figure}
